# Supplementary material for: Fully Fine-tuned CLIP Models are Efficient Few-Shot Learners
Source: arXiv:2407.04003 source file (2024-07-04)
Supplement: Supplementary file 1 [file appendix.tex]

\section{Supplementary Materials}









% This section contains supplementary material that provides additional details for the main paper and further experimental analysis. The content of this section is as follows:
% \begin{itemize}
%     \item Additional Experimental Details
%     \item Additional Experimental Analysis
%     \item Additional Ablation Study
% \end{itemize}

\subsection{Additional Experimental Details}

\textbf{Competitors}
We compare the proposed approach with the related competitors, i.e., CLIP, CoOp, CoCoOp, MaPLe, and CLIPood, ranging from prompt learning and fine-tuning methods. The details of competitors are as follows: 
\begin{itemize}
    \item \textbf{CLIP.} \cite{clip} CLIP is a vision model trained on web-scale data (400 million) with exceptional zero-shot reasoning capability as well as its generalization ability. CLIP consists of an image encoder and a text encoder, which are trained together with a contrastive pre-training process.
    \item \textbf{CoOp.} \cite{coop} CoOp uses the prompt engineering method to adapt a vision-language model like CLIP to downstream tasks by simply adding learnable context to build the prompt.
    \item \textbf{CoCoOp.} \cite{cocoop} CoCoOp introduces a lightweight network structure based on CoOp to generate an input-specific token which helps the model overcome the overfitting issue.
    \item \textbf{MaPLe.} \cite{maple} MaPLe introduces stage-wise text prompt and vision prompt to the text encoder as well as the image encoder of CLIP to better align the vision-language representations of the model. Also, this approach proposes a coupling function to ensure synergy between both modalities.
    \item \textbf{CLIPood.} \cite{clipood} CLIPood introduces the margin metric softmax as a novel training objective for fine-tuning the model. Additionally, it utilized the Beta moving average to generate ensemble weights, synthesizing the pre-trained and fine-tuned models.
\end{itemize}

\textbf{Dataset Details.} In \cref{tab:detail-datasets}, we list the details of the datasets and the hand-crafted prompt we used in the experiments. The prompts are from the \cite{clip} and we have not adopted more prompt templates to generate the optical text representations. In this work, we only focus on the effect of fully fine-tuned CLIP and the text representations would be automatically learned during the training.

\textbf{Training Details.}
We maintain the temperature of the softmax function consistent with the pre-trained model, using $\tau$ = 0.01, except for when $\mathcal{L}_{VLD}$ is adjusted to 0.1. All images are randomly resized and cropped to 224 × 224, only random resize and random crop data augments are applied. The optical hyper-parameter $\lambda$ is set to 0.7, $\eta$ is set to 0.1, and $\alpha$ is set to 0.5 for all experiments. We use the AdamW optimizer with the cosine learning rate strategy and the learning rate is set to 5e-6 and trained for 20 epochs. The batch size is set to 32 for most datasets, with specific batch sizes of 16 for EuroSAT and 64 for ImageNet. For each result of CLIP-CITE, we report the average result with three random seeds.

\begin{table*}[!htb]
    \centering
    % \resizebox{\linewidth}{!}{
        \begin{tabular}{lccccc}
        \toprule
        Dataset & Classes & Train & Val & Test & Hand-crafted Prompt \\
        \midrule
        Caltech101 & 100 & 4,128 & 1,649 & 2,465 & a photo of a [CLS]. \\
        OxfordPets & 37 & 2,944 & 736 & 3,669 & a photo of a [CLS], a type of pet. \\ 
        StanfordCars & 196 & 6,509 & 1,635 & 8,041 & a photo of a [CLS]. \\
        Flowers102 &  102 & 4,093 & 1,633 & 2,463&  a photo of a [CLS], a type of flower. \\
        Food101 &  101 & 50,500 & 20,200 & 30,300 & a photo of [CLS], a type of food. \\
        FGVCAircraft &  100 & 3,334 & 3,333 & 3,333 & a photo of a [CLS], a type of aircraft. \\
        SUN397 &  397 & 15,880 & 3,970 & 19,850 & a photo of a [CLS]. \\
        DTD &  47 & 2,820 & 1,128 & 1,692 & [CLS] texture.\\
        EuroSAT &  10 & 13,500 & 5,400 & 8,100 & a centered satellite photo of [CLS]. \\
        UCF101 &  101 & 7,639 & 1,898 & 3,783 & a photo of a person doing [CLS].\\
        ImageNet &  1,000 & 1.28M & N/A & 50,000 & a photo of a [CLS] \\
        \midrule
        ImageNetV2	& 1,000	& N/A	& N/A	& 10,000 &  a photo of a [CLS] \\
        ImageNet-Sketch	& 1,000	& N/A	& N/A	& 50,889 &  a photo of a [CLS] \\
        ImageNet-A	& 200	& N/A	& N/A	& 7,500 &  a photo of a [CLS] \\
        ImageNet-R	& 200	& N/A	& N/A	& 30,000  & a photo of a [CLS] \\
        \bottomrule
        \end{tabular}    
    % }
    \caption{Detailed statistics of the datasets.}
    \label{tab:detail-datasets}
\end{table*}

\begin{figure}[!tb]
    \centering
    \includegraphics[width=\linewidth]{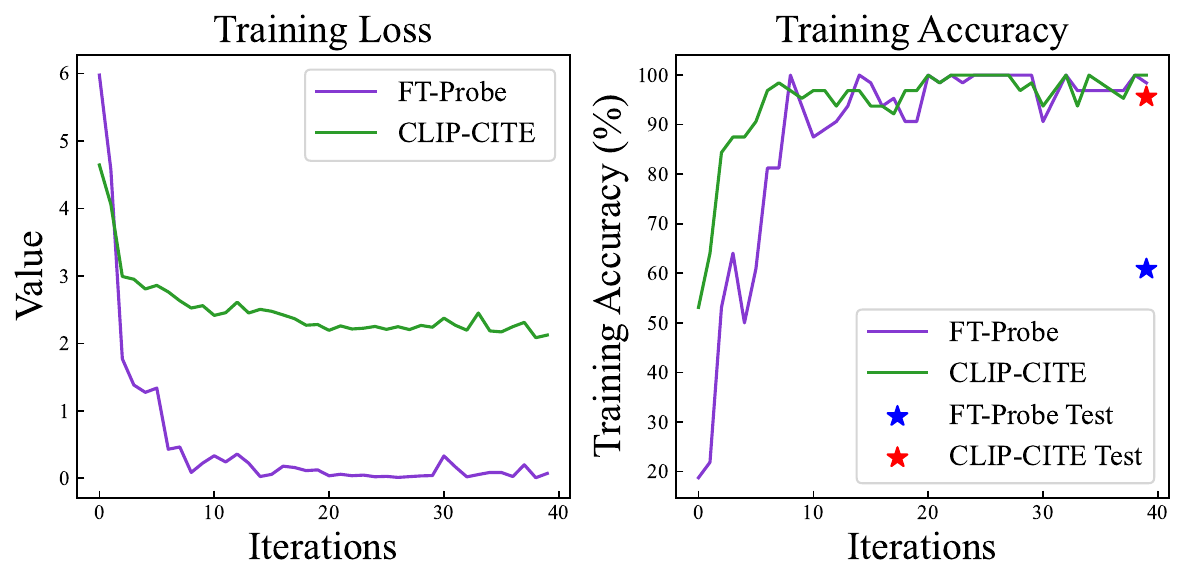}
    \caption{Training loss and accuracy of FT-Probe and CLIP-CITE on EuroSAT dataset.}
    \vspace{-0.8mm}
    \label{fig:loss}
\end{figure}

\subsection{Additional Experimental Analysis}
\textbf{Overfitting analysis.} We demonstrate the training process of \textbf{FT-Probe} and our \textbf{CLIP-CITE} illustrated in \cref{fig:ft-methods} on EuroSAT dataset. The results of loss and accuracy of the training dataset are shown in \cref{fig:loss}. We observe that, for the FT-Probe model, there is a decline in the training loss, accompanied by a continual increase in accuracy on the training set. However, the final accuracy on the test set is only 60.86\%, which suggests the occurrence of overfitting. In contrast, in the case of our CLIP-CITE model, there is also a reduction in the loss function and a consistent rise in training set accuracy, culminating in a test set accuracy of 95.61\%. This indicates that our approach does not exhibit overfitting, demonstrating effectiveness. Moreover, it highlights that overcoming overfitting is a crucial issue when fully fine-tuning models.

\subsection{Additional Ablation Study}

\textbf{Prompt Learning with proposed loss.} To evaluate the effectiveness of full-fine-tuning, we also explore the prompt learning methods with our proposed loss. The results, detailed in \cref{tab: PL + different objectives}, indicate that prompt learning methods experience a modest improvement with the implementation of our proposed loss functions \textit{i.e.} $L_{SCL}$ and $L_{VLD}$. Notably, our CLIP-CITE still maintains a performance edge. Besides, with the simple fine-tuning (FT-Probe), the tuned model seems to be overfitting, as shown in \cref{fig:ft-methods}. Therefore, we propose that both full fine-tuning and well-designed loss functions are crucial in adapting VLMs to the downstream few-shot tasks.

\begin{table}[!h]
    \centering
    \resizebox{0.98\linewidth}{!}{
        \begin{tabular}{l@{\hspace{0.8cm}}c@{\hspace{0.8cm}}c@{\hspace{0.3cm}}|@{\hspace{0.3cm}}c@{\hspace{0.8cm}}c@{\hspace{0.8cm}}c}
        \toprule
        Method &  $\mathcal{L}_{SCL}$ & $\mathcal{L}_{VLD}$ & \footnotesize{B} & \footnotesize{N} & \footnotesize{HM }\\
        \midrule
            CLIP  & & & 72.43 & 68.14 & 70.22 \\
        \midrule
             CoOp & & & 76.47 & 67.88 & 71.92 \\
             CoOp & \checkmark & & 76.51 & 67.93 & 71.97 \\
             CoOp & \checkmark & \checkmark & 78.23 & 70.89 & 72.11 \\
        \midrule
             MaPLe & & & 76.66 & 70.54 & 73.47 \\
             MaPLe & \checkmark & & 76.70 & 70.67 & 73.56 \\
             MaPLe & \checkmark & \checkmark & 76.71 & 70.89 & 73.69 \\ 
        \midrule
             CLIP-CITE & \checkmark & \checkmark & 78.44 & 71.07 & 74.58 \\
        \bottomrule
        \end{tabular}
    }
    \vspace{-0.2cm}
    \caption{Ablation results (\%) of our CLIP-CITE and prompt learning with various training objectives on the BNG task of the ImageNet dataset.}
    \label{tab: PL + different objectives}
\end{table}

\textbf{The effect of the hyper-parameter $\lambda$ and $\eta$.} In \cref{fig:hyperparam}, we ablate the different values on $\lambda$ and $\eta$ in \cref{eq:total-loss}. From the results, we observe that the performances in terms of HM are better when applying the $\mathcal{L}_{SCL}$, e.g., $\lambda$ is greater than 0. It indicates that supervised vision-language alignment is necessary when fine-tuning. Besides, the vision-language similarity distillation can regularize the model well when $\eta$ is less than 0.1. In the experiments, the optical $\lambda$ and $\eta$ are set to 0.7 and 0.1, respectively.

\begin{figure}[!tb]
% \vspace{cm} 
\centering
\subfloat[The effect of $\lambda$.]{
\begin{tikzpicture}
\pgfplotsset{every axis legend/.append style={at={(0.5,1.03)}, anchor=south},every axis y label/.append style={at={(0.15,0.5)}}, every axis x label/.append style={at={(0.5,0.06)}}}
\begin{axis}[xtick={0.0,0.2, 0.5,0.7,1.0},legend columns=4,legend style={font=\tiny},font=\scriptsize,width=5cm]
\addplot table [x=lambda, y=Base, col sep=comma] {lambda.csv};
\addplot table [x=lambda, y=New, col sep=comma] {lambda.csv};
\addplot table [x=lambda, y=HM, col sep=comma] {lambda.csv};
\legend{Base, New, HM}
\end{axis}
\end{tikzpicture}}
\subfloat[The effect of $\eta$.]{
\begin{tikzpicture}
\pgfplotsset{every axis legend/.append style={at={(0.5,1.03)},
anchor=south}, every axis x label/.append style={at={(0.5,0.06)}}}
\begin{axis}[xtick={0,0.3,0.5,0.7,1.0},xticklabels={0,0.05,0.1,0.3,0.5},legend columns=3,legend style={font=\tiny},font=\scriptsize,width=5cm]
\addplot table [x=eta, y=Base, col sep=comma] {eta.csv};
\addplot table [x=eta, y=New, col sep=comma] {eta.csv};
\addplot table [x=eta, y=HM, col sep=comma] {eta.csv};
\legend{Base, New, HM}
\end{axis}
\end{tikzpicture}}
\vspace{-2mm}
\caption{The impacts of the hyper-parameter $\lambda$ and $\eta$ on the base-to-new generalization performances. We report the  Base (\%), New (\%), and HM (\%) accuracy on the ImageNet dataset.}
\label{fig:hyperparam}
\end{figure}

\begin{figure}[!h]
   \begin{overpic}[width=\linewidth]{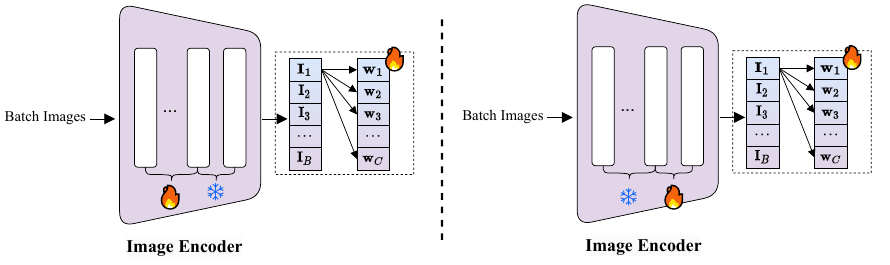} 
   \vspace{10mm}
   \scriptsize
   \put(6, -2){(a)~Fine-tuning previous layers.}
   \put(58, -2){(b)~Fine-tuning late layers.}
   \end{overpic}
   \vspace{1mm}
   \caption{Illustration of fine-tuned model within the distinct layers. (a) illustrates layers preceding the image encoder, while (b) delineates layers succeeding the image encoder.}
   \label{fig:ft-ratio}
\end{figure}

\begin{figure}[!htb]
    \centering
        \subfloat[The effect of fine-tuning previous layers and freezing the late $i_{th}$ layers.]{
    \begin{tikzpicture}
    \pgfplotsset{every axis legend/.append style={at={(0.5,1.03)}, minimum width=1.4cm,anchor=south,font=\fontsize{6}{8}\selectfont},every axis y label/.append style={at={(0.15,0.5)}}, every axis x label/.append style={at={(0.5,0.06)}}}
    \begin{axis}[xlabel={i},xlabel style={font=\small},legend columns=4,legend style={font=\small},font=\scriptsize,width=8cm,height=5cm]
    \addplot table [x=frozen, y=Base, col sep=comma] {after_frozen.csv};
    \addplot table [x=frozen, y=New, col sep=comma] {after_frozen.csv};
    \addplot table [x=frozen, y=HM, col sep=comma] {after_frozen.csv};
    \legend{Base, New, HM}
    \end{axis}
    \end{tikzpicture}}   \\
    \vspace{3mm} 
    \subfloat[The effect of fine-tuning late layers and freezing the previous $i_{th}$ layers.]{
    \begin{tikzpicture}
    \pgfplotsset{every axis legend/.append style={at={(0.5,1.03)}, minimum width=1.4cm, anchor=south, font=\fontsize{6}{8}\selectfont},every axis y label/.append style={at={(0.15,0.5)}}, every axis x label/.append style={at={(0.5,0.06)}}}
    \begin{axis}[xlabel={i},xlabel style={font=\small},legend columns=4,legend style={font=\small},font=\scriptsize,width=8cm,height=5cm]
    \addplot table [x=frozen, y=Base, col sep=comma] {before_frozen.csv};
    \addplot table [x=frozen, y=New, col sep=comma] {before_frozen.csv};
    \addplot table [x=frozen, y=HM, col sep=comma] {before_frozen.csv};
    \legend{Base, New, HM}
    \end{axis}
    \end{tikzpicture}}   
    \caption{The effect of the fine-tuning layers. (a) indicates we fine-tune the previous layers and freeze the $i_{th}$  late layers corresponding to \cref{fig:ft-ratio}. (a), while (b) indicates we freeze the previous $i_{th}$ layers and fine-tune the late layers corresponding to \cref{fig:ft-ratio}. (b). }
    \label{fig:frozen-layer}
\end{figure}

% \begin{figure}
%     \centering
%     \begin{tabular}{cc}
%     \includegraphics[width=0.3\linewidth]{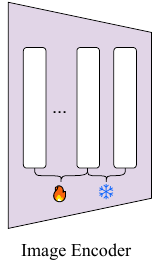} & 
%     \includegraphics[width=0.3\linewidth]{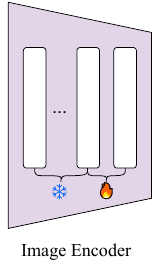} \\
%     \end{tabular}
%     \caption{Caption}
%     \label{fig:enter-label}
% \end{figure}

\begin{figure*}[!ht]
    % \centering
    % \vspace{-0.2cm}
     \setlength{\tabcolsep}{0pt}
     \def\mywidth{.25}
     %\begin{subfigure}{\linewidth}
     \begin{tabular}{cccc}
     % c@{\hskip 5pt}c@{\hskip 15pt}c@{\hskip 15pt}c
     \includegraphics[width=\mywidth\linewidth]{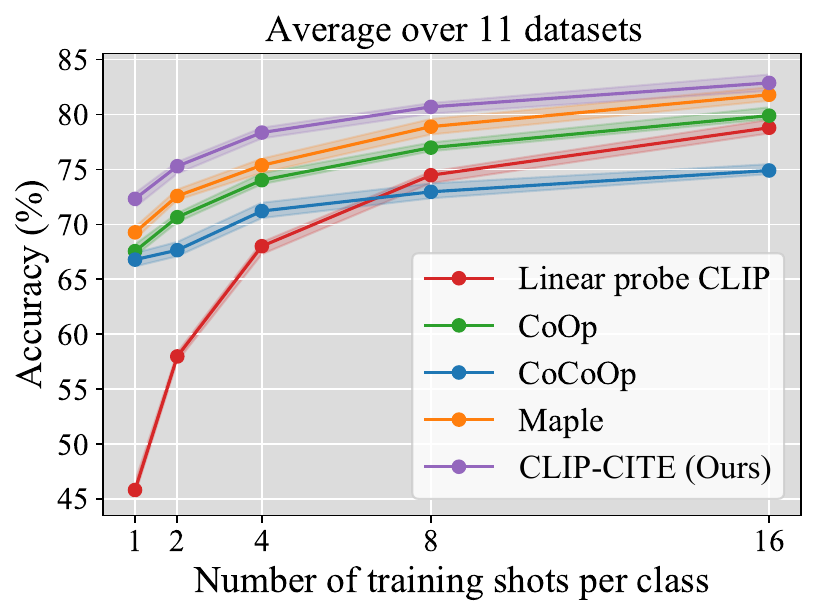} &
     \includegraphics[width=\mywidth\linewidth]{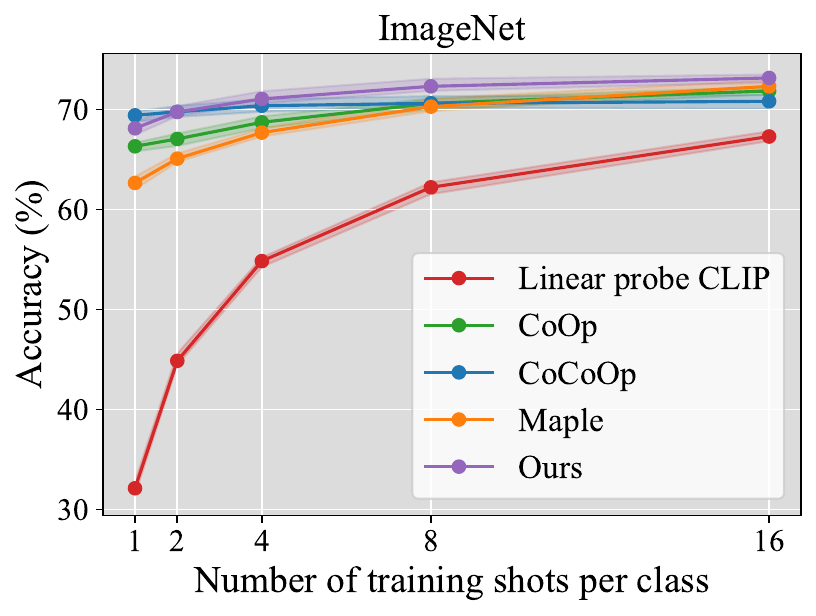} &
      \includegraphics[width=\mywidth\linewidth]{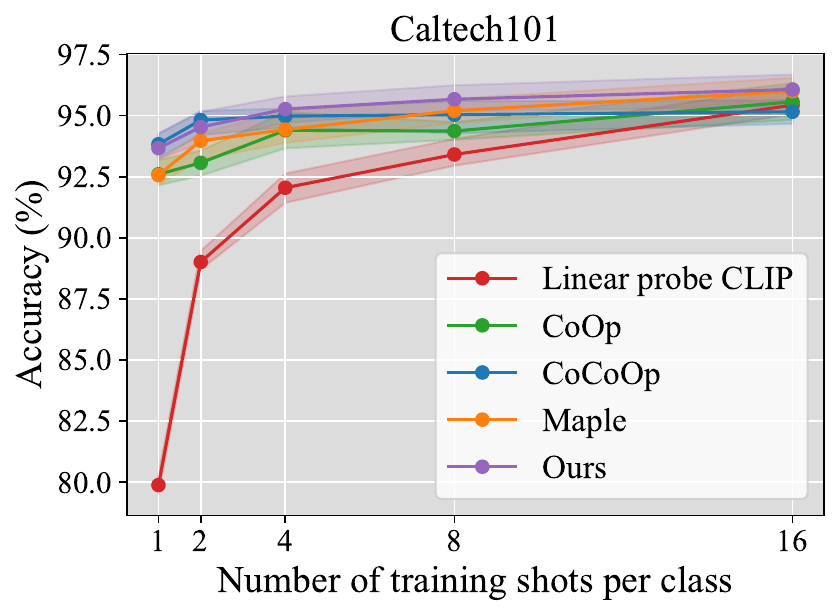} &
      \includegraphics[width=\mywidth\linewidth]{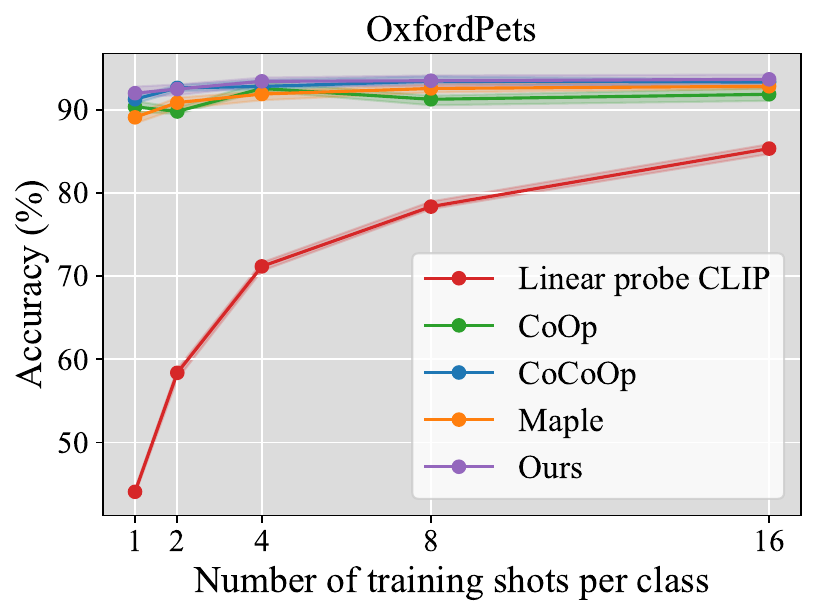} \\
      % \vspace{-0.2cm}
     \includegraphics[width=\mywidth\linewidth]{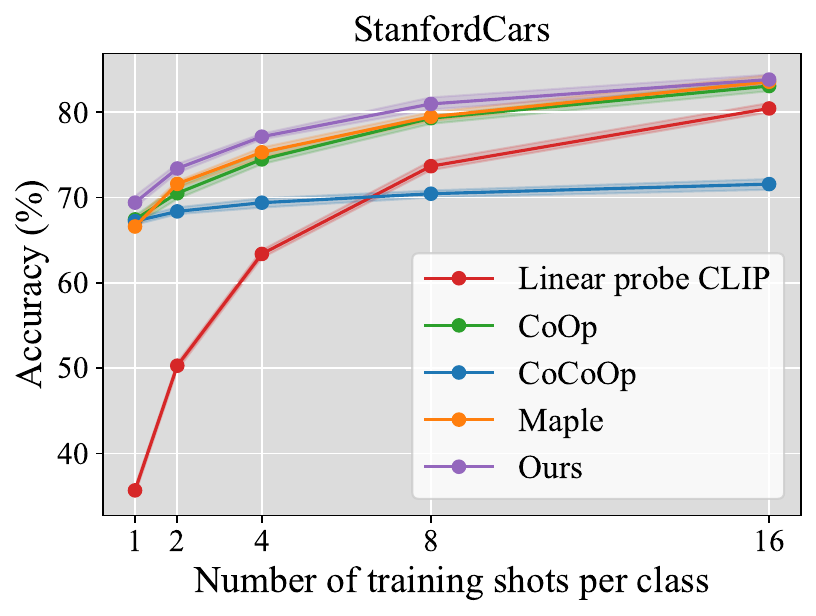} &
     \includegraphics[width=\mywidth\linewidth]{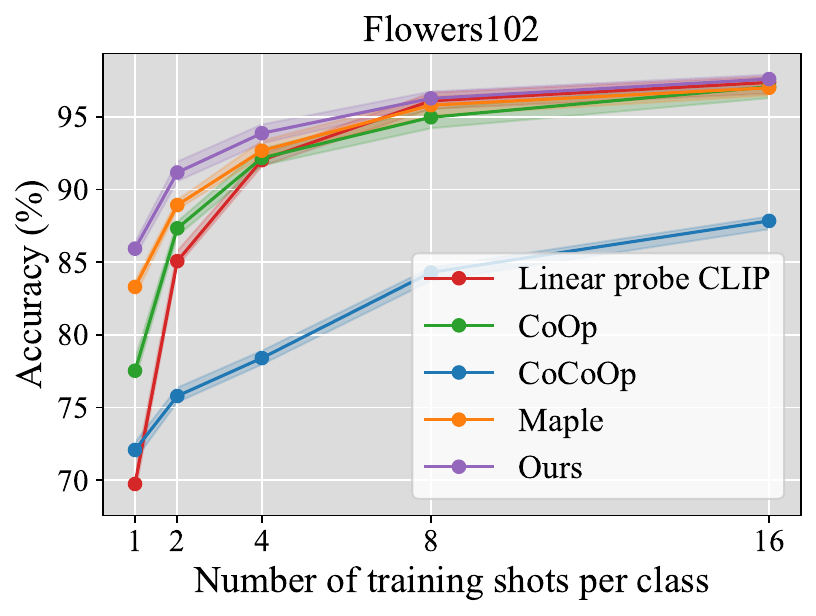} &
      \includegraphics[width=\mywidth\linewidth]{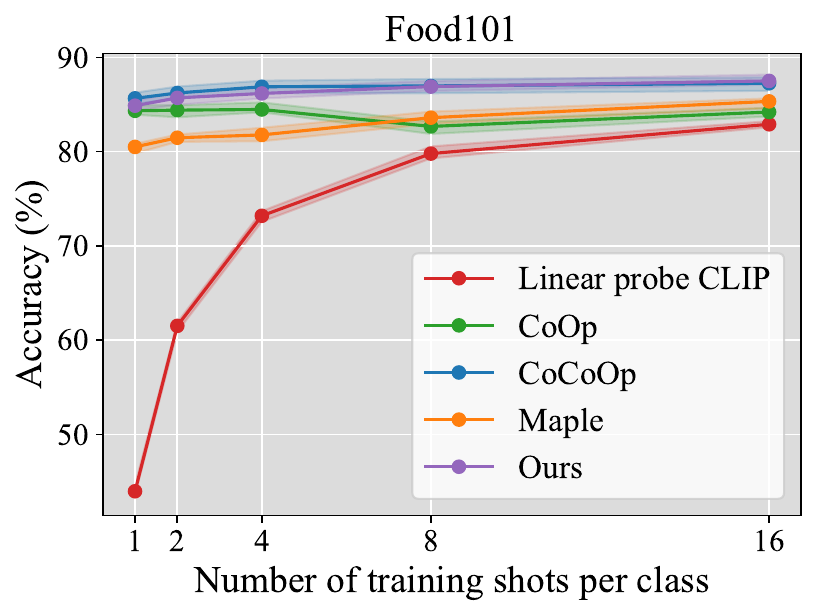} &
      \includegraphics[width=\mywidth\linewidth]{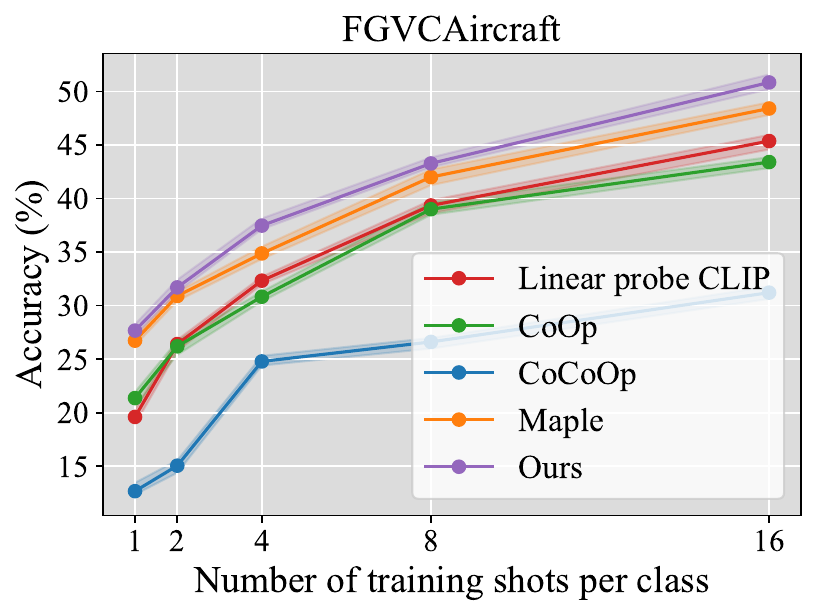} \\
      % \vspace{-0.2cm}
     \includegraphics[width=\mywidth\linewidth]{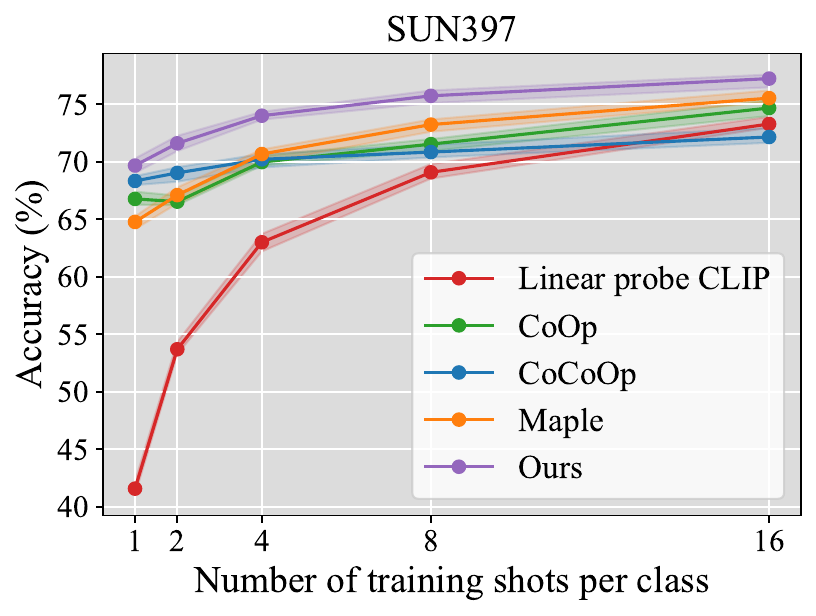} &
     \includegraphics[width=\mywidth\linewidth]{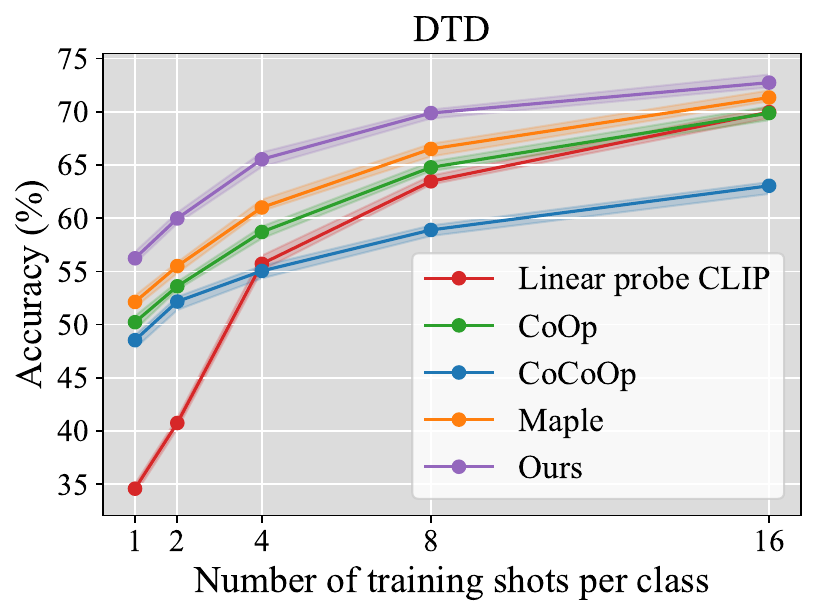} &
      \includegraphics[width=\mywidth\linewidth]{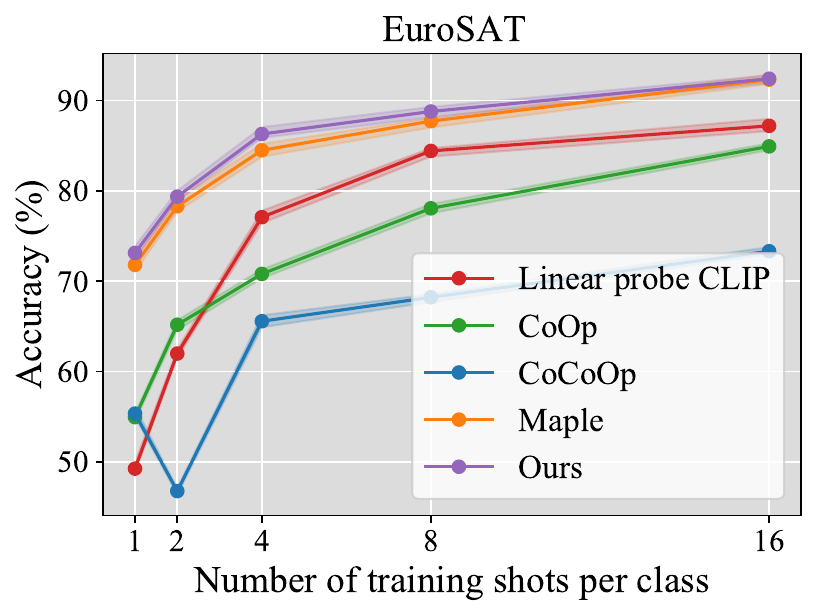} &
      \includegraphics[width=\mywidth\linewidth]{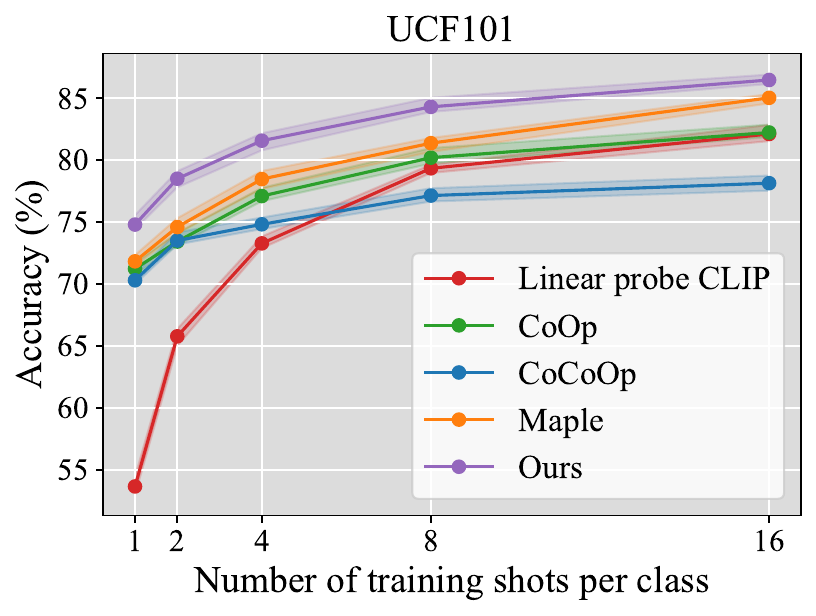} \\      
     \end{tabular}
     \vspace{-0.2cm}
    \caption{Comparison results of few-shot learning benchmark on the 11 datasets. All of the methods are trained on the ViT-B/16 backbone and implemented with the same experimental settings.}
   \label{fig:fsl-every-datasets}
\end{figure*}

\textbf{The effect of the full fine-tuning.} \cref{fig:ft-ratio} shows the different fine-tuning manners of the image encoder, \textit{e.g.} fine-tuning previous layers and fine-tuning late layers. And we conduct the experiments with $\mathcal{L}_{DVA}$ for ablation. \cref{fig:frozen-layer}. (a) shows the results that we fine-tune previous layers and freeze the late layers, while \cref{fig:frozen-layer}. (b) the results that we fine-tune previous layers and freeze the late layers. From the experimental results, we observe that when there are only a few frozen layers, the performance is comparable to full fine-tuning. However, as the number of frozen layers increases, the effectiveness diminishes, \textit{i.e.} the last 3 frozen layers led to a decline in the results shown in \cref{fig:frozen-layer}. (a). Overall, full fine-tuning is better than partial fine-tuning.

\textbf{The effect of weights ensemble ratio $\alpha$.} \cref{tab:alpha} shows the results of different datasets with the different ensemble ratios $\alpha$. Without weights ensemble, CLIP-CITE achieves 85.79\%, 73.52\%, and 79.19\% in Base, New, and HM accuracy, respectively. With the fine-tuning weights ensemble, the performance increases from 71.70\% to 78.90\% in HM accuracy when $\alpha$ is 0.1. When $\alpha$ increases, the Base accuracy increases, and the New accuracy fluctuates slightly. The optimal value $\alpha$ appears to be 0.5. This indicates that our fine-tuning process maintains a subtle change of model parameters, facilitating smooth compatibility with the zero-shot pre-trained CLIP model and resulting in an overall enhancement of effectiveness.

\textbf{More experimental results of Cross-Domain setting.} \cref{tab:imagenet-to} and \cref{tab:to-imagenet} shows the experimental results of Cross-Domain setting.  From the results of \cref{tab:imagenet-to}, all methods trained on the ImageNet can consistently obtain the generalization performance on the other 10 datasets. From the results of \cref{tab:to-imagenet}, the prompt learning methods trained on other datasets are difficult to transfer to ImageNet and impact the overall generalization, while our fine-tuning methods can maintain or even enhance the performance of ImageNet. These demonstrate that ImageNet encompasses a broader array of patterns and categories, and both prompt learning methods and our approach effectively sustain performance across various datasets. When transferring from other datasets to ImageNet, CLIP-CITE can uphold ImageNet's performance. It shows that our fine-tuning method has better generalization capacity.

\textbf{The quantitive details of few-shot learning benchmark.} \cref{fig:fsl-every-datasets} shows the detailed results of each dataset in the few-shot learning settings. Totally, our method achieves a considerable gain on all shots of the dataset.

% \begin{table}[]
%     \centering
%     \begin{tabular}{c|c}
%          &  \\
%          & 
%     \end{tabular}
%     \caption{Caption}
%     \label{tab:my_label}
% \end{table}

% \begin{figure}[!htb]
%     \centering
%     \includegraphics[width=\linewidth]{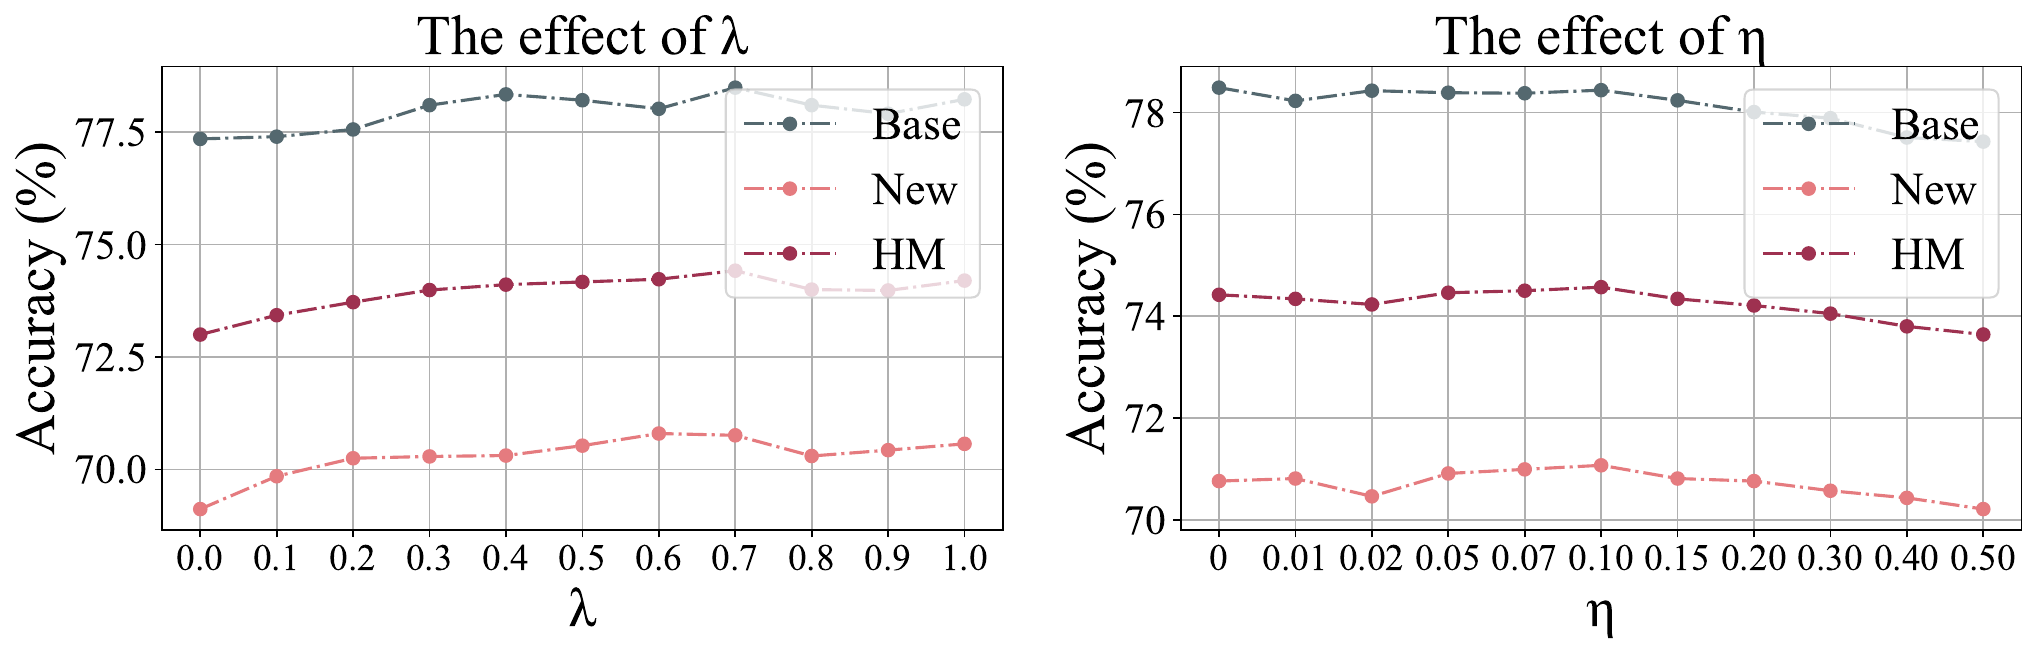}
%     \caption{The impacts of the hyper-parameter $\lambda$ and $\eta$ to the base-to-new generalization performances on ImageNet.}
%     \label{fig:lambda-beta}
% \end{figure}

\begin{table*}[]
    \centering
    % \resizebox{\linewidth}{!}{
        \begin{tabular}{c|cc|cc|cc|cc|cc}
        \toprule
        \multirow{2}{*}{Methods}  & \multicolumn{2}{c|}{CLIP} & \multicolumn{2}{c|}{CoOp} & \multicolumn{2}{c|}{CoCoOp}  & \multicolumn{2}{c|}{MaPLe}  & \multicolumn{2}{c}{CLIP-CITE} \\
        \cmidrule{2-11}
         & Base & New & Base & New & Base & New & Base & New & Base & New \\
        \midrule
        Caltech101 & 96.84 & 94.00 & 94.15 & 93.92 & 96.58 & 95.16 & 96.30 & 94.98 & 96.71 & 93.82 \\
        OxfordPets & 91.17 & 97.26 & 90.34 & 97.69 & 90.8 & 97.97 & 90.57 & 97.73 & 89.56 & 96.78 \\
        StanfordCars & 63.37 & 74.89 & 61.99 & 73.37 & 63.62 & 74.48 & 62.44 & 73.98 & 60.74 & 72.41 \\
        Flowers102 & 72.08 & 77.80 & 66.86 & 75.23 & 72.30 & 77.64 & 73.25 & 76.86 & 71.48 & 76.9 \\
        Food101 & 90.10 & 91.22 & 88.62 & 90.68 & 89.39 & 91.0 & 89.29 & 90.86 & 88.47 & 90.53 \\
        FGVCAircraft & 27.19 & 36.29 & 21.21 & 26.36 & 27.65 & 32.37 & 28.69 & 31.21 & 26.33 & 34.33 \\
        SUN397 & 69.36 & 75.35 & 68.36 & 72.78 & 72.08 & 75.96 & 71.46 & 76.1 & 71.78 & 76.16 \\
        DTD & 53.24 & 59.90 & 49.00 & 51.73 & 55.32 & 57.01 & 51.04 & 54.51 & 50.39 & 57.53 \\
        EuroSAT & 56.48 & 64.05 & 50.2 & 69.22 & 52.1 & 68.84 & 47.52 & 59.83 & 49.50 & 65.51\\
        UCF101 & 70.53 & 77.50 & 68.89 & 71.88 & 70.89 & 75.77 & 69.22 & 74.97 & 70.99 & 76.55 \\
        \bottomrule        
        \end{tabular}
    % }
    \caption{Cross-Domain evaluation. All the models are trained on the base training set of the ImageNet dataset and evaluated on the 10 datasets .}
    \label{tab:imagenet-to}
\end{table*}

\begin{table*}[!tb]
    \centering
    \resizebox{\linewidth}{!}{
        \begin{tabular}{lc|ccccc>{\columncolor{gray!20}}cccccc}
        \toprule
        \multicolumn{2}{c|}{$\alpha$ ratio} & 0 & 0.1 & 0.2 & 0.3 & 0.4 & \textbf{0.5} & 0.6 & 0.7 & 0.8 & 0.9 & 1.0 \\
        % &  & [\cite{clip}] & [\cite{coop}] & [\cite{cocoop}] & [\cite{maple}]  & [\cite{clipood}] &  \\
        \midrule 
        \multirow{3}{*}{Average on} & Base & 69.34 & 83.53 & 84.66 & 84.44 & 85.09 & 85.48 & 85.64 & 85.69 & 85.64 & 85.58 & 85.79 \\
        & New &74.22&74.75&76.07&75.71&75.74&77.08&74.68&75.58&75.62&75.77&73.52 \\
        & HM &71.70&78.90&80.13&79.83&80.15&81.06&79.79&80.32&80.32&80.38&79.19 \\        
        \midrule  
        \multirow{3}{*}{ImageNet}          &     Base&72.43&77.45&77.63&78.20&78.23&78.44&78.44&78.48&78.46&78.49&78.50 \\
&New&68.14&70.35&70.79&70.71&70.65&71.07&70.32&70.59&70.36&70.29&70.23 \\
&HM&70.22&73.73&74.05&74.27&74.25&74.58&74.16&74.33&74.19&74.17&74.14 \\
        \midrule
        \multirow{3}{*}{Caltech101}     &         Base&96.84&97.20&97.65&97.78&98.77&98.82&98.82&98.83&98.83&98.83&98.85 \\
& New&94.00&93.40&94.14&93.44&93.65&94.28&93.53&93.90&94.00&93.47&93.20 \\
& HM&95.40&95.26&95.86&95.56&96.14&96.50&96.10&96.30&96.36&96.08&95.94 \\

        \midrule
        \multirow{3}{*}{OxfordPets}  & Base&91.17&95.23&95.84&95.66&95.82&96.01&96.18&96.42&96.60&96.93&97.01 \\
        & New&97.26&96.12&96.47&96.69&96.71&97.95&96.66&96.72&96.90&97.28&95.23 \\
        & HM&94.12&95.67&96.15&96.17&96.27&96.97&96.42&96.57&96.75&97.11&96.11 \\
        
        \midrule
        \multirow{3}{*}{Stanford Cars}       &     Base&63.37&80.13&81.49&81.00&81.70&82.83&83.00&82.86&82.98&82.94&83.01 \\
& New&74.89&72.34&74.17&73.83&72.96&74.51&72.45&72.70&71.21&70.96&70.23 \\
& HM&68.65&76.04&77.65&77.25&77.08&78.45&77.37&77.45&76.65&76.48&76.09 \\
        \midrule
        \multirow{3}{*}{Flowers102}        &      Base&72.08&94.23&95.32&94.61&95.25&95.98&96.21&96.04&96.18&96.16&96.23 \\ 
& New&77.80&75.30&76.08&75.39&75.30&76.45&72.31&75.02&73.94&74.92&71.36 \\
& HM&74.83&83.71&84.62&83.91&84.11&85.11&82.57&84.24&83.61&84.22&81.95 \\
        \midrule
        \multirow{3}{*}{Food101}   &             Base&90.10&90.43&90.78&90.73&90.74&90.81&90.25&90.74&90.68&90.24&90.23 \\
& New&91.22&90.84&91.48&91.17&90.86&91.55&90.17&90.18&91.10&91.37&89.27 \\
& HM&90.66&90.63&91.15&90.54&90.80&91.18&90.21&90.46&90.89&90.80&89.75 \\

        \midrule
        \multirow{3}{*}{FGVC\\Aircraft}    &    Base&27.19&43.01&45.24&44.19&46.52&47.26&49.14&49.61&48.79&47.70&50.23 \\
& New&36.29&36.23&36.77&37.91&37.14&38.37&35.36&36.80&35.82&37.99&35.35 \\
& HM&31.09&39.33&40.57&40.81&41.31&42.35&41.12&42.25&41.31&42.30&41.50 \\

        \midrule
        \multirow{3}{*}{SUN397}         &          Base&69.36&80.13&81.90&81.73&81.95&82.30&82.26&82.18&82.30&82.18&82.10 \\
& New&75.35&77.50&79.02&78.51&78.52&79.40&78.72&78.69&78.71&78.96&78.23 \\
& HM&72.23&78.79&80.43&80.09&80.20&80.82&80.45&80.40&80.46&80.54&80.12 \\

        \midrule
        \multirow{3}{*}{DTD}            &          Base&53.24&82.30&83.45&83.64&83.68&84.26&83.81&83.68&83.64&83.95&83.02 \\
& New&59.90&60.23&63.56&64.01&62.47&64.54&61.36&58.76&62.89&60.05&58.30 \\
& HM&56.37&69.56&72.16&72.52&71.53&73.09&70.85&69.04&71.79&70.02&68.50 \\ 

        \midrule
        \multirow{3}{*}{EuroSAT}          &       Base&56.48&92.34&95.34&94.12&95.77&95.61&96.17&95.99&96.01&95.96&96.45 \\
&New&64.05&72.45&75.47&72.70&76.90&80.59&72.44&80.26&77.88&79.59&70.23 \\
&HM&60.03&81.19&84.25&82.04&85.31&87.46&82.64&87.42&86.00&87.01&81.28 \\

        \midrule
        \multirow{3}{*}{UCF101} & Base&70.53&86.34&86.67&87.13&87.54&87.56&87.80&87.77&87.58&88.03&88.10 \\
        & New&77.50&77.50&78.76&78.43&78.03&79.01&78.20&77.83&78.99&78.61&77.12 \\
& HM&73.85&81.68&82.53&82.55&82.51&83.07&82.72&82.50&83.06&83.05&82.25 \\
        \bottomrule    
        \end{tabular}   
    }
   \caption{Comparison with the different ensemble ratio $\alpha$ on base-to-new generalization.}
   \label{tab:alpha}
\end{table*}

\begin{table*}[!htb]
    \centering
    \resizebox{0.65\linewidth}{!}{
    \begin{tabular}{c|c|ccccc}
    \toprule
    Dataset & Method & 1-shot & 2-shot & 4-shot & 8-shot & 16-shot \\
    \midrule
    \multirow{5}{*}{Average} &  Linear probe CLIP & 45.83 &57.98&68.01&74.47&78.79\\
    & CoOp & 67.56&70.65&74.02&76.98&79.89\\
    & CoCoOp & 66.79&67.65&71.21&72.96&74.90\\
    & MaPLe&69.27&72.58&75.37&78.89&81.79\\
    & CLIP-CITE &72.69&75.58&77.85&80.62&83.31 \\
    \midrule
    \multirow{5}{*}{ImageNet} & Linear probe CLIP	& 32.13&44.88&54.85&62.23&67.31 \\
    &  CoOp	& 66.33&67.07&68.73&70.63&71.87 \\ 
    & CoCoOp	& 69.43&69.78&70.39&70.63&70.83 \\
    & MaPLe	& 62.67&65.10&67.70&70.30 & 72.33 \\ 
    & CLIP-CITE  	& 68.20&68.90&70.30&71.20&72.90 \\
    \midrule
    \multirow{5}{*}{Caltech101} & Linear probe CLIP	& 79.88&89.01&92.05&93.41&95.43 \\
    & CoOp	& 92.60&93.07&94.4& 94.37 & 95.57 \\ 
    & CoCoOp	& 93.83&94.82&94.98 & 95.04& 95.16 \\
    & MaPLe	& 92.57&93.97&94.43&95.2&96.00 \\
    & CLIP-CITE 	& 94.16&94.81&95.53&96.39&96.50 \\
    \midrule
    \multirow{5}{*}{OxfordPets} & Linear probe CLIP& 44.06&58.37&71.17&78.36&85.34 \\
    & CoOp	& 90.37&89.8&92.57&91.27&91.87 \\
    & CoCoOp	& 91.27&92.64&92.81&93.45&93.34 \\ 
    & MaPLe	& 89.10 & 90.87&91.9&92.57&92.83 \\
    & CLIP-CITE 	& 91.47&93.02&93.54&93.87&94.70 \\    
    \midrule
    \multirow{5}{*}{StanfordCars} & Linear probe CLIP& 35.66&50.28&63.38&73.67&80.44\\
    & CoOp	& 67.43&70.5&74.47&79.3&83.07\\
    & CoCoOp	& 67.22&68.37&69.39&70.44&71.57\\
    & MaPLe	& 66.60&71.60&75.30&79.47&83.57\\
    & CLIP-CITE 	& 70.63&74.22&76.53&79.94&83.70\\    
    \midrule
    \multirow{5}{*}{Food101} & Linear probe CLIP	& 43.96	& 61.51	& 73.19	& 79.79	& 82.90\\
        & CoOp	& 84.33& 	84.40	& 84.47& 	82.67& 	84.20\\
        & CoCoOp	& 85.65& 	86.22& 	86.88	& 86.97	& 87.25\\
        & MaPLe	& 80.50	& 81.47	& 81.77	& 83.60	& 85.33\\
        & CLIP-CITE 	& 85.16	& 85.95	& 86.05	& 86.68	& 87.00\\    
    \midrule
    \multirow{5}{*}{Flowers102} & Linear probe CLIP	& 69.74	& 85.07	& 92.02	& 96.10	& 97.37\\
    & CoOp	& 77.53	& 87.33	& 92.17	& 94.97	& 97.07\\
    & CoCoOp & 72.08	& 75.79	& 78.40 & 	84.30 & 	87.84\\
    & MaPLe	& 83.30	& 88.93	& 92.67& 	95.80& 	97.00\\
    & CLIP-CITE 	& 84.25	& 86.76	& 92.08	& 95.86	& 97.6 \\    
    \midrule
    \multirow{5}{*}{FGVCAircraft} & Linear probe CLIP	& 19.61	& 26.41	& 32.33	& 39.35	& 45.36\\
& CoOp	& 21.37	& 26.20	& 30.83	& 39.00	& 43.40 \\
& CoCoOp	& 12.68	& 15.06	& 24.79	& 26.61	& 31.21\\
& MaPLe	& 26.73	& 30.90	& 34.87	& 42.00	& 48.40 \\
& CLIP-CITE 	& 29.34	& 32.40	& 36.60	& 46.00	& 57.00 \\    
    \midrule
    \multirow{5}{*}{SUN397} & Linear probe CLIP	& 41.58	& 53.70	& 63.00	& 69.08	& 73.28\\
    & CoOp	& 66.77	& 66.53	& 69.97	& 71.53	& 74.67\\
    & CoCoOp	& 68.33	& 69.03	& 70.21	& 70.84	& 72.15\\
    & MaPLe	& 64.77	& 67.10	& 70.67	& 73.23	& 75.53\\
    & CLIP-CITE 	& 69.54	& 70.99	& 72.36	& 74.45	& 76.30\\    
    \midrule
    \multirow{5}{*}{DTD} & Linear probe CLIP	& 34.59	& 40.76	& 55.71	& 63.46	& 69.96\\
    & CoOp	& 50.23	& 53.60	& 58.70	& 64.77	& 69.87\\
    & CoCoOp	& 48.54	& 52.17& 	55.04	& 58.89	& 63.04\\
    & MaPLe	& 52.13	& 55.50	& 61.00	& 66.50 & 	71.33\\
    & CLIP-CITE 	& 54.20	& 60.70	& 64.54	& 67.67	& 72.50\\    
    \midrule
    \multirow{5}{*}{EuroSAT} & Linear probe CLIP	& 49.23	& 61.98	& 77.09	& 84.43	& 87.21\\
& CoOp& 	54.93	& 65.17& 	70.80& 	78.07	& 84.93\\
& CoCoOp& 	55.33	& 46.74	& 65.56	& 68.21	& 73.32\\
& MaPLe	& 71.80& 	78.30	& 84.50	& 87.73& 	92.33\\
& CLIP-CITE 	& 76.20	& 85.20& 	88.77	& 91.17	& 92.60 \\        
    \midrule
    \multirow{5}{*}{UCF101} & Linear probe CLIP	& 53.66	& 65.78	& 73.28	& 79.34	& 82.11\\
        & CoOp& 	71.23& 	73.43& 	77.10& 	80.20& 	82.23 \\
        & CoCoOp	& 70.30& 	73.51	& 74.82	& 77.14& 	78.14\\
        & MaPLe& 	71.83& 	74.60	& 78.47& 	81.37	& 85.03\\
        & CLIP-CITE 	& 76.40& 	78.38	& 80.07	& 83.56	& 85.70 \\        
    \bottomrule        
    \end{tabular}    
    }
    \caption{Per-dataset performance comparison of our method with various methods in the few-shot setting.}
    \label{tab:per-dataset}
\end{table*}
